# Supplementary material for: Explosive Legged Robotic Hopping: Energy Accumulation and Power Amplification via Pneumatic Augmentation
Source: arXiv:2312.05773 source file (2023-12-10)
Supplement: Supplementary file 1 [file Appendix.tex]

\section*{APPENDIX}
\begin{table}[h]
    \centering
    \caption{The physical parameters of the robot}
    \label{tab:robot_parameters}
    \begin{tabular}{ccc} 
        \toprule
        Parameters  & Value [unit] \\
        \midrule
        Shank length $l_s$ & 100 mm \\
        Thigh length $l_t$ & 150 mm \\
        Stroke of pump $d_p$ & 130 mm \\
        Stroke of actuator $d_a$ & 101.6 mm \\
        %Angle between the pump and actuator and the shank & 45° \\
        %Angle between the pump and actuator and the Thigh & 45° \\
        \midrule
        Motor maximum torque $\tau_m$ & 3.728 Nm\\  
        Motor maximum speed $\omega_m$ & 223 rpm\\
        \bottomrule
    \end{tabular}
\end{table}
